# Supplementary material for: Computing secure key rates for quantum key distribution with untrusted devices
Source: arXiv:1908.11372 source file (2021-11-03)
Supplement: Supplementary file 1 [file supp.pdf]

# Supplementary Information:
# Computing secure key rates for quantum cryptography with untrusted devices

## I. EVE'S SIDE-INFORMATION AS ENTROPY PRODUCTION

We first give a more detailed derivation of the relation described in the main text between $H(A_0|E)$ and entropy production on $\rho_{AB}$. Following the notation in the main text, recall that our goal is to find a lower bound on

$$\begin{aligned} &\inf H(A_0|E) \\ &\text{s.th. } \langle X_{ab|xy}\rangle_{\psi_{ABE}} = \Pr(ab|xy), \end{aligned} \tag{1}$$

where $X_{ab|xy} = P_{a|x} \otimes P_{b|y}$, and the infimum takes place over $\psi_{ABE}$ and any measurements. (In the main text, a slightly more general situation was considered, where constraints were formed using linear combinations of the operators $X_{ab|xy}$; note that subsequent analyses in this Supplement can be easily generalized to that situation.) In Sec. V below, we argue that without loss of generality, we can assume that all uncharacterized measurements are projective.

We regard the process of producing Alice's raw key (in one round) as a quantum-to-classical channel $R$ that maps Alice's quantum system $A$ to a memory register $A_0$ that stores the classical measurement outcome. Explicitly, we have

$$R[\rho] = \sum_a |a\rangle\langle a| \operatorname{tr}(\rho P_{a|0}). \tag{2}$$

By considering the complementary channel of $R\otimes \mathrm{id}_B$, we can express $H(A_0|E)$ in terms of $\rho_{AB}$ using the following lemma:

**Lemma 1.** *For any projective measurement $A_0$ on a pure state $\psi_{ABE}$ as described above, we have*

$$H(A_0|E) = H\left(T\left[\rho_{AB}\right]\right) - H\left(\rho_{AB}\right), \tag{3}$$

*where $T$ is the pinching channel*

$$T[\rho_{AB}] = \sum_a (P_{a|0} \otimes \mathbb{I}_B)\rho_{AB}(P_{a|0} \otimes \mathbb{I}_B). \tag{4}$$

*If all projectors $P_{a|0}$ are rank-1, this reduces to*

$$H(A_0|E) = H(A_0|B) - H(A|B). \tag{5}$$

*Proof.* By Stinespring's theorem [1], we can describe the channel $R$ as the restriction of an isometry $V$ from $A$ to an expanded system $A_0A'$. For projective measurements, we can take $A'$ to be isomorphic to $A$ and use

$$V|\psi\rangle_A = \sum_a |a\rangle_{A_0} \otimes P_{a|0}|\psi\rangle_A, \tag{6}$$

as easily verified by a short calculation.

When this isometry is applied to Alice's part of our initial global pure state $\Psi_{ABE}$, it maps it to a pure final state $\Psi_{A'BEA_0}$. Since the entropies of the two sides of a bipartite pure state are equal, we have

$$H(E) = H(AB) \text{ and } H(A_0E) = H(A'B), \tag{7}$$

and hence we can write

$$\begin{aligned} H(A_0|E) &= H(A_0E) - H(E) \\ &= H(A'B) - H(AB) \\ &= H(T[\rho_{AB}]) - H(\rho_{AB}), \end{aligned} \tag{8}$$

where $T$ is the complementary channel of $R \otimes \mathrm{id}_B$:

$$\begin{aligned} T[\rho_{AB}] &= \operatorname{tr}_{A_0}((V\otimes \mathbb{I}_B)\rho_{AB}(V^*\otimes \mathbb{I}_B)) &(9)\\ &= \sum_a (P_{a|0} \otimes \mathbb{I}_B)\rho_{AB}(P_{a|0} \otimes \mathbb{I}_B). &(10) \end{aligned}$$

If all measurement operators are rank-1 projectors, we can write them in the form $P_{a|0} = |a\rangle\langle a|_A$ and identify these with the register states $|a\rangle\langle a|_{A_0}$, in which case $T[\rho_{AB}] \cong \rho_{A_0B}$ and hence the expression simplifies to

$$\begin{aligned} H(T[\rho_{AB}]) - H(\rho_{AB}) &= H(A_0B) - H(AB) &(11)\\ &= H(A_0|B) - H(A|B), &(12) \end{aligned}$$

as claimed. □

We remark that if one is instead interested in lower-bounding the entropy $H(A_0B_0|E)$ of *both* Alice and Bob's outputs (for inputs $(x, y) = (0, 0)$), the proof of Lemma 1 also generalizes to that task, by constructing

$$V|\psi\rangle_{AB} = \sum_{ab} |ab\rangle_{A_0B_0} \otimes (P_{a|0} \otimes P_{b|0})|\psi\rangle_{AB}, \tag{13}$$

$$T[\rho_{AB}] = (P_{a|0} \otimes P_{b|0})\rho_{AB}(P_{a|0} \otimes P_{b|0}). \tag{14}$$

(This slightly increases the order of the operator polynomial $K$ in our subsequent constructions.) Such a bound is used in, for instance, security proofs for DI randomness expansion [2]. However, additional work would seem to be necessary to obtain bounds suitable for DI randomness *amplification*, where the biased input distribution can increase the Bell value achievable by classical (insecure) models.

Additionally, the analysis generalizes to POVMs (i.e. a set of operators $E_{a|0} \geq 0$ such that $\sum_a E_{a|0} = \mathrm{id}_A$) as well, though in that case we would choose $A'$ to be isomorphic to $A_0'A$ where $A_0'$ is a copy of $A_0$, and take

$$V|\psi\rangle_A = \sum_a |aa\rangle_{A_0A_0'} \otimes \sqrt{E_{a|0}}|\psi\rangle_A, \tag{15}$$

$$T[\rho_{AB}] = \sum_a |a\rangle\langle a|_{A_0'} \otimes M_{a|0}\rho_{AB}M_{a|0}, \tag{16}$$

where $M_{a|0} := \left(\sqrt{E_{a|0}} \otimes \mathbb{I}_B\right)$.

## II. BOUNDING THE ENTROPY PRODUCTION

Having reduced our task to bounding the entropy production, we introduce the following ansatz: given a quantum channel $T$ and a self-adjoint operator $L$, we aim to find an operator $K$ such that

$$H\left(T[\rho]\right) - H(\rho) \geq \langle L \rangle_\rho - \ln\langle K \rangle_\rho \tag{17}$$

holds on all quantum states. Any valid solution to (17) will allow us to lower-bound the entropy production of $T$ by estimating the expectations of $K$ and $L$. The form of the ansatz (17) arises from our use of the Gibbs variational principle (see Lemma 2), though it can also be viewed as arising from the Lagrange dual of the optimization in 1. (In Sec. VI we give a more detailed analysis of the dual, from which we find that our approach yields bounds that are essentially tight up to the use of the generalised Golden–Thompson inequality and NPA hierarchy. Also, at the end of that section we show that our approach yields a convex bound, which is relevant for applying the entropy accumulation theorem [2–4].) For brevity, we will for now denote the constraints $\left\langle X_{ab|xy} \right\rangle = \Pr(ab|xy)$ in the form $\langle X_j \rangle = \gamma_j$ for $j$ in an index set $\mathcal{J}$.

For simplicity we will assume that all measurements act on finite dimensional systems. However, our bounds will be completely independent of this dimension, and hence can be considered device-independent since they do not need any explicit bound on the system dimensions. Additionally, we will assume that all measurements have a countable set of possible outcomes. Note that this assumption only puts a relatively mild restriction to applicability: firstly, we cover all projective measurements on finite-dimensional systems. By this we already cover a big part of the typical measurement settings considered in literature, e.g. spin measurements, discrete energy levels, and anything that happens in a quantum computer. In addition, one can always argue that continuous sets of outcomes are "only" an idealized object: in an experiment, continuous sets are typically coarse-grained by sorting outcomes into a finite set of bins.

Nevertheless, from our perspective, an extension of this work to continuous sets of outcomes and/or infinite-dimensional systems seems possible. However, we will leave this for future work since it would require an extension of some of the theorems used, such as the extended Golden–Thompson inequality of [5], to integrals (in place of sums) and/or infinite-dimensional operators, which would go beyond the scope of this work.

Our main result, which we prove in Sec. IV, provides a family of possible choices of $K$:

**Proposition 1.** *Let $T$ be a quantum channel with adjoint $T^*$. For any set of self-adjoint operators $\tilde{L}_j$, the operators $L$ and $K$ defined as*

$$L = \sum_j \tilde{L}_j, \tag{18}$$

$$K = T^* T\left[\int_{\mathbb{R}} dt\, \beta(t) \left|\prod_j e^{\frac{1+it}{2}\tilde{L}_j}\right|^2\right], \tag{19}$$

$$\text{with } \beta(t) = \frac{\pi/2}{\cosh(\pi t) + 1}, \tag{20}$$

*satisfy Eq. (17)*[1] *for all quantum states $\rho$. (We use the notation $|A|^2 = A^* A$.)*

There is a considerable amount of freedom in choosing the operators $\tilde{L}_j$. In particular, we can choose $\tilde{L}_j = \lambda_j X_j$ for any coefficients $\lambda_j \in \mathbb{R}$. These coefficients would in general play the role of variational parameters that can be used to optimize the bound (17) in a particular situation (in fact they can be interpreted as Lagrange multipliers, see Sec. VI). With this choice of $L_j$, we can directly write down the expectation of $L$ as

$$\langle L \rangle_\rho = \sum_j \lambda_j \gamma_j. \tag{21}$$

It therefore only remains to bound the expectation of $K$ in order to evaluate the r.h.s of (17).

For the device-dependent case, Prop. 1 will allow us represent $K$ as an explicit matrix whenever representations of the $X_j$ are known, since in this case the integration in (19) can be solved analytically (see Eqs. (25)–(26)). Then bounding $\langle K \rangle_\rho = \mathrm{tr}(\rho K)$ via the constraints imposed by the observed values is precisely an SDP:

$$\begin{aligned} \max \quad & \mathrm{tr}(\rho K) \\ \text{s.th.:} \quad & \mathrm{tr}(\rho X_j) = \gamma_j \quad \forall j \in \mathcal{J} \\ & \mathrm{tr}(\rho) = 1 \\ & \rho \geq 0 \end{aligned} \tag{22}$$

As a further feature, a solution of (22) also allows us to judge the quality of our bound: an SDP solver used for (22) should additionally provide an optimizer $\rho^*$, which is a valid quantum state that satisfies the constraints $\langle X_j \rangle_{\rho^*} = \gamma_j$. Hence it will give a feasible point for our original optimization (Eq. (1)). We can then compute the value of the objective function at that feasible point, and compare it with our lower bound to quantify the quality of our bound for a given set of variational parameters $\lambda_j$.

For the device-independent case, the measurement operators $X_j$ are not known, but we shall now describe how Prop. 1 can still be applied. As previously mentioned, we can assume that all $X_j$ are projectors (though not necessarily rank-1). It is also convenient to assume that these

[1] All entropies are in base $e$ unless otherwise specified.

projectors can be relabelled as $X_{k|l}$ such that for each value of $l$, the operators $X_{k|l}$ form a resolution of the identity, i.e. $\sum_k X_{k|l} = \mathbb{I}$ and $X_{k|l}X_{k'|l} = \delta_{kk'}X_{k|l}$. (This would automatically be true if the constraints include the probabilities of all outcomes from every measurement; otherwise, it could always be achieved in principle by introducing an extra projector $X_j' = \mathbb{I} - X_j$ for each $X_j$.) Then for any scalars $c_{k|l} \in \mathbb{C}$, it holds that

$$\exp\left(\sum_k c_{k|l}X_{k|l}\right) = \sum_k e^{c_{k|l}}X_{k|l}, \tag{23}$$

which directly yields the following corollary by choosing $\tilde{L}_l = \sum_k \lambda_{k|l}X_{k|l}$ in Prop. 1:

**Corollary 1.** *Let $T$ be a quantum channel with adjoint $T^*$. Take any family of projectors $X_{k|l}$ such that for each $l$, we have $\sum_k X_{k|l} = \mathbb{I}$ and $X_{k|l}X_{k'|l} = \delta_{kk'}X_{k|l}$. Then for any coefficients $\lambda_{k|l} \in \mathbb{R}$, the operators $L$ and $K$ defined as*

$$L = \sum_{kl} \lambda_{k|l}X_{k|l}, \tag{24}$$

$$K = T^*T\left[\int_{\mathbb{R}} dt\, \beta(t) \left|\prod_l \left(\sum_k e^{\frac{1+it}{2}\lambda_{k|l}}X_{k|l}\right)\right|^2\right], \tag{25}$$

*satisfy Eq. (17) for all quantum states $\rho$.*

Theorem 1 in the main text can be obtained from this corollary by using the fact that the channel $T$ in that scenario satisfies $T^*T = T$, followed by replacing $X_{k|l}$ with $P_{a|x} \otimes P_{b|y}$ and $\lambda_{k|l}$ with $\sum_j \lambda_j c^{(j)}_{abxy}$.

To use Eq. (25) in practice, we need to simplify it further, by expanding the product and evaluating the integrals via the result[2] $\int_{\mathbb{R}} dt\, e^{i\alpha t}\beta(t) = \alpha \operatorname{csch}\alpha$ for $\alpha \in \mathbb{R}$. Supposing that $l \in \{1, 2, \dots, N\}$ and recalling our notation $|A|^2 = A^*A$, this gives

$$\begin{aligned} K &= T^*T\left[\int_{\mathbb{R}} dt\, \beta(t) \sum_{\substack{k_1,\dots,k_N,\\ k_1',\dots,k_N'}} \exp\left(\sum_{l=1}^N \left(\frac{1-it}{2}\lambda_{k_l'|l} + \frac{1+it}{2}\lambda_{k_l|l}\right)\right) X_{k_N'|N}\dots X_{k_1'|1}X_{k_1|1}\dots X_{k_N|N}\right] \\ &= \sum_{\substack{k_1,\dots,k_N,\\ k_1',\dots,k_N'}} e^{\alpha^+_{\boldsymbol{kk}'}}\, \alpha^-_{\boldsymbol{kk}'} \operatorname{csch}\alpha^-_{\boldsymbol{kk}'}\; T^*T\left[X_{k_N'|N}\dots X_{k_1'|1}X_{k_1|1}\dots X_{k_N|N}\right], \text{ where } \alpha^\pm_{\boldsymbol{kk}'} = \sum_{l=1}^N \frac{\lambda_{k_l|l} \pm \lambda_{k_l'|l}}{2}. \end{aligned} \tag{26}$$

The sum can be further simplified slightly by using $X_{k_1|1}X_{k_1'|1} = \delta_{k_1k_1'}X_{k_1|1}$ to eliminate the summation over $k_1'$. The indices $\{1, 2, \dots, N\}$ can be permuted to yield other possible choices of $K$.

Note that even without grouping the operators $X_j$ into resolutions of the identity, a similar result still holds for coefficients $\lambda_j \in \mathbb{R}$ by choosing $\tilde{L}_j = \lambda_j X_j$, in which case the operator product could be written as

$$\left|\prod_j \left(\left(e^{\frac{1+it}{2}\lambda_j} - 1\right)X_j + \mathbb{I}\right)\right|^2. \tag{27}$$

When the operators can be grouped into resolutions of the identity, this reduces to the expression in (25) as long as the operator product does not break up the groupings.

We now note that as long as the Kraus operators of the channel $T^*T$ are polynomials in the measurement operators, Eq. (26) is such a polynomial as well. This is an important property, because the task of maximizing $\langle K\rangle_\rho$ over all possible measurement operators is now a non-commutative polynomial optimisation similar to the type studied in [6]. (For completeness, in Sec. VII we will briefly collect the essential steps and assumptions that are needed to bound this optimization via an SDP hierarchy, as described in that work.)

[2] The expression $\alpha \operatorname{csch}\alpha$ should be interpreted as having the removable discontinuity at $\alpha = 0$ "filled in", i.e. take $\alpha \operatorname{csch}\alpha = 1$ at $\alpha = 0$ (this correctly matches the evaluation of the integral for $\alpha = 0$). To evaluate the integral for $\alpha \neq 0$, note that since $e^{i\alpha t}\beta(t) = (\pi/4)e^{i\alpha t}\operatorname{sech}^2(\pi t/2)$, the integral is absolutely convergent and hence we can evaluate it by finding its Cauchy principal value. Due to the $\operatorname{sech}^2(\pi t/2)$ factor, the integrand is holomorphic on $\mathbb{C}$ except at $\{(2m+1)i \mid m \in \mathbb{Z}\}$, where it has poles of order 2. The integral can then be evaluated by using a rectangular contour with corners at $\pm R$ and $\pm R + 2i$ (which encloses one pole) and taking $R \to \infty$.

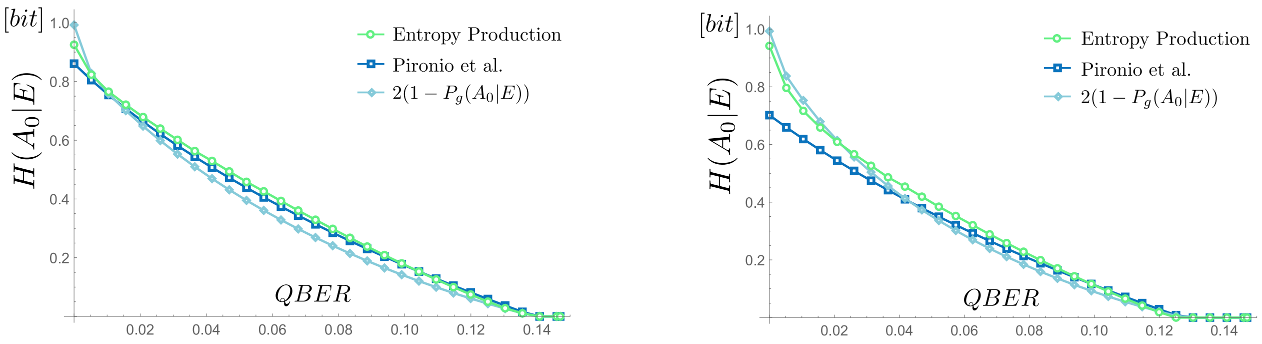


FIG. 1. **Tilted CHSH inequalities:** Lower bounds on $H(A_0|E)$ (in base 2) as a function of depolarizing noise applied to distributions maximizing the tilted CHSH value [7]. The plots on the left and right are for $\alpha = 1.5$ and $\alpha = 2$ respectively (see Eq. (28)). Our approach yields better results than previous methods for some values of depolarizing noise.

## III. NUMERICAL BOUNDS ON $H(A_0|E)$

The channel $T$ relevant for DIQKD (Eq. (4)) indeed has the property that the Kraus operators of $T$ are explicit polynomials in the measurement operators, allowing us to apply the above results[3]. We can hence apply our method to bound $H(A_0|E)$ in various DI and sDI scenarios, which we now describe. In the following, all optimization of the coefficients $\vec{\lambda}$ was done numerically, so it is possible that there exist choices of coefficients that yield better bounds but were not found by the numerical methods. (In Sec. VIII, we provide more details on our numerical approaches, including some methods to simplify the task.)

First, as described in the main text, we considered depolarizing-noise and limited-detection-efficiency models for distributions that maximize the CHSH value. We performed calculations for those scenarios at level 6 of the NPA hierarchy (see Sec. VIII). Also, note that the limited-detection-efficiency model does not produce uniform distributions for $A_0$, but we still wish to apply the inequality[1] $H(A_0|E) \geq (2\ln 2)(1 - P_g(A_0|E))$ [8], which was derived for uniform $A_0$. This can be addressed by performing a symmetrization step [9, 10], which produces a distribution with uniform $A_0$. The value of $H(A_0|E)$ before symmetrization is lower-bounded by the value after symmetrization (following the argument in [10] with von Neumann entropy in place of min-entropy), so it suffices to bound $P_g(A_0|E)$ for the latter and use it to bound $H(A_0|E)$.

As for the bounds on the two-party entropy $H(A_0B_0|E)$, they were computed by choosing the channel $T$ as described in Eq. (14). This entropy is the relevant quantity for describing the asymptotic key rate for randomness expansion [3], and a finite-size analysis against non-IID attacks can also be performed using entropy accumulation as described in that work. We note that these improved bounds on $H(A_0B_0|E)$ could also slightly improve the key rates for DIQKD security proofs based on entropy accumulation, because part of the proof involves the two-party entropy rather than the one-party entropy. (Specifically, the key rate can be improved by an amount on the order of the test-round probability.)

In addition, we also consider 2-input 2-output distributions that maximally violate tilted CHSH inequalities [7] of the form

$$\alpha\left(\langle A_0B_0\rangle + \langle A_0B_1\rangle\right) + \langle A_1B_0\rangle - \langle A_1B_1\rangle. \tag{28}$$

It was shown in [7] that as $\alpha \to \infty$, these distributions become arbitrarily close to the set of local distributions but still certify that $H(A_0|E) = 1$. However, this result was only derived at maximal violation of the tilted CHSH inequalities, i.e. in the absence of noise. When noise is applied to these distributions, the only existing method to robustly bound $H(A_0|E)$ is the suboptimal $P_g(A_0|E)$-based approach. As shown in Fig. 1, we find that for $\alpha = 1.5$ and $\alpha = 2$, our method outperforms this approach in most noise regimes (and also the CHSH-based bound, since the CHSH violation for these distributions becomes arbitrarily small at large $\alpha$). However, note that at any fixed value of $q$, choosing measurements such that the distribution maximizes the CHSH value (instead of the tilted CHSH value) under this noise model currently still yields better bounds on $H(A_0|E)$ than applying our approach to these distributions, at least for these values of $\alpha$.

Finally, we consider a 4-input 2-output distribution obtained by performing the Pauli measurements[4]

$$\begin{aligned} A_0 = B_0 = Z, \quad A_1 = B_1 = (X+Z)/\sqrt{2}, \\ A_2 = B_2 = X, \quad A_3 = B_3 = (X-Z)/\sqrt{2}, \end{aligned} \tag{29}$$

[3] There is in fact additional structure in the DIQKD setting due to the tensor-product form $X_{ab|xy} = P_{a|x} \otimes P_{b|y}$, but this only comes into play when applying the NPA hierarchy.

[4] This can be viewed as having Alice and Bob perform each other's "standard CHSH measurements" in addition to their own.

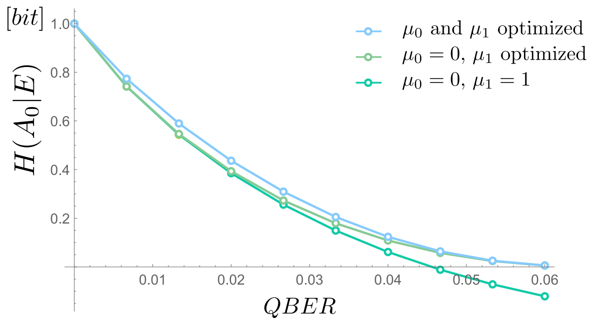


FIG. 2. **4-input 4-output DI scenario:** Lower bounds on $H(A_0|E)$ (in base 2) as a function of depolarizing noise, for the distribution produced by the measurements (29) on a Werner state. Here we do not optimize all the coefficients $\vec{\lambda}$ in Corollary 1, but only choose them such that they yield an entropic uncertainty relation in the form of lower bounds on $H(A_0|E)+\mu_0 H(A_0|B_0)+\mu_1 H(A_1|B_1)$, for various choices of $\mu_0$ and $\mu_1$ as specified in the diagram. However, it can be seen that the resulting bounds are not very robust against noise.

on the Werner state $(1-2q)|\Phi^+\rangle\langle\Phi^+| + (q/2)\mathbb{I}$. As the matrices in the NPA hierarchy are substantially larger for this scenario, we could not apply our method in its full generality. Instead, we only considered a special case where the coefficients $\vec{\lambda}$ are chosen such that $\langle L\rangle_\rho = \mu_0 H(A_0|B_0) + \mu_1 H(A_1|B_1)$, for two free parameters $\mu_0, \mu_1$ to be optimized over (this can be viewed as yielding an entropic uncertainty relation in the form of lower bounds on $H(A_0|E)+\mu_0 H(A_0|B_0)+\mu_1 H(A_1|B_1)$). This substantially reduces the order of the polynomial in Eq. (26), since the product only involves two pairs of $(x, y)$ values, and hence NPA level 3 suffices to bound $\langle K\rangle_\rho$ in this case.[5] As shown in Fig. 2, this allows us to certify $H(A_0|E) = 1$ in the absence of noise (where $H(A_0|B_0) = H(A_1|B_1) = 0$ for this distribution), with the optimum at that point being attainable by $\mu_1 = 1$ and, apparently, arbitrary $\mu_0 \geq 0$ (negative values of $\mu_0$ appear to yield worse bounds as $|\mu_0|$ increases). However, the bound is not very robust as the noise level increases—presumably, we would need to include more measurement operators in $L$ to obtain more robust bounds. We were also unable to further improve it by numerically optimizing over all the parameters $\lambda_{ab|00}, \lambda_{ab|11}$ instead of simply $\mu_0, \mu_1$.

We remark that choosing $\langle L\rangle_\rho = \mu_1 H(A_1|B_1)$ for the 2-input 2-output scenarios in the main text results in a suboptimal bound that only certifies $H(A_0|E) \geq 0.398$ in the absence of noise. We also used this choice of $\langle L\rangle_\rho$ to investigate distributions numerically optimized to maximize violation of the I4422 inequality [11], but were only able to find the same suboptimal bound even after optimizing over all $\lambda_{ab|00}$. This may possibly be related to the fact that for these distributions we have $H(A_1|B_1) \neq 0$ even in the absence of noise.

[5] As long as the operator product ordering is chosen such that the operators $X_{ab|00}$ are placed at the end of the product.

## IV. PROOF OF THE MAIN RESULT

To prove our main proposition (Prop. 1) we will make use of the following lemmas, the proofs of which we provide for completeness:

**Lemma 2.** *(Gibbs variational principle) Let $C$ be a self-adjoint operator. Then for all quantum states $\rho$,*

$$-\operatorname{tr}(\rho C) \geq H(\rho) - \ln \operatorname{tr}\left(e^C\right). \tag{30}$$

*Proof.* Consider the thermal state $\sigma = e^C/\operatorname{tr}(e^C)$. We have

$$\begin{aligned} -\operatorname{tr}(\rho C) &= -\operatorname{tr}\left(\rho \ln e^C\right) \\ &= -\operatorname{tr}\left(\rho \ln \frac{e^C}{\operatorname{tr}(e^C)}\right) - \ln \operatorname{tr}\left(e^C\right) \\ &= -\operatorname{tr}\left(\rho \ln \sigma\right) - \ln \operatorname{tr}\left(e^C\right) \\ &\geq H(\rho) - \ln \operatorname{tr}\left(e^C\right), \end{aligned} \tag{31}$$

where the last line follows from non-negativity of relative entropy: $\operatorname{tr}(\rho\ln\rho - \rho\ln\sigma) = D(\rho||\sigma) \geq 0$. □

**Lemma 3.** *(An extended Golden–Thompson inequality, given as a sub-case of Corollary 3.3 in [5]) Let $C_1, C_2, \ldots, C_N$ be finite-dimensional self-adjoint operators. We have the inequality*

$$\operatorname{tr}\left(e^{\sum_j C_j}\right) \leq \int_{\mathbb{R}} dt\ \beta(t) \operatorname{tr}\left(\left|\prod_j e^{\frac{1+it}{2}C_j}\right|^2\right). \tag{32}$$

*(The inequality holds for all orderings of the operator product.)*

*Proof.* Let $||C||_p = \operatorname{tr}(|C|^p)^{1/p}$ denote the Schatten $p$-norm of an operator $C$. We first note that since all $C_j$ are self-adjoint, we have

$$\operatorname{tr}\left(e^{\sum_j C_j}\right) = \operatorname{tr}\left(\left|e^{\sum_j C_j/2}\right|^2\right) = \left\|e^{\sum_j C_j/2}\right\|_2^2. \tag{33}$$

Corollary 3.3 in [5] states that for all $p \geq 1$,

$$\ln\left\|e^{\sum_j C_j/2}\right\|_p \leq \int_{\mathbb{R}} dt\ \beta(t) \ln\left\|\prod_j e^{(1+it)C_j/2}\right\|_p. \tag{34}$$

Taking logarithms on both sides of Eq. (33) and applying

this inequality for $p=2$, we find

$$\begin{aligned}\ln\operatorname{tr}\left(e^{\sum_j C_j}\right) &= 2\ln\left\|e^{\sum_j C_j/2}\right\|_2 \\ &\leq 2\int_{\mathbb{R}} dt\;\beta(t)\ln\left\|\prod_j e^{\frac{1+it}{2}C_j}\right\|_2 \\ &= \int_{\mathbb{R}} dt\;\beta(t)\ln\operatorname{tr}\left(\left|\prod_j e^{\frac{1+it}{2}C_j}\right|^2\right) \\ &\leq \ln\int_{\mathbb{R}} dt\;\beta(t)\operatorname{tr}\left(\left|\prod_j e^{\frac{1+it}{2}C_j}\right|^2\right)\end{aligned} \tag{35}$$

where the last line follows from concavity of the logarithm. Since the logarithm is also monotone increasing, this implies the desired result. □

We now prove our main result, Prop. 1.

*Proof.* Starting from (17) we want to find $K$ such that

$$H\left(T[\rho]\right) - \langle L\rangle_\rho - H(\rho) \geq -\ln\langle K\rangle_\rho \tag{36}$$

holds on all states $\rho$. To do so, first we use Jensen's operator inequality to write

$$H\left(T[\rho]\right) \geq -\operatorname{tr}\left(\rho\ln\left(T^*T[\rho]\right)\right), \tag{37}$$

since ln is concave. We combine this with Lemma 2 with the substitution $C = \ln\left(T^*T[\rho]\right) + L$:

$$\begin{aligned}&H\left(T[\rho]\right) - \langle L\rangle_\rho - H(\rho) \\ &\geq -\operatorname{tr}\left(\rho\left(\ln\left(T^*T[\rho]\right)+L\right)\right) - H(\rho) \\ &\geq -\ln\left(\operatorname{tr}\left(e^{\ln(T^*T[\rho])+L}\right)\right).\end{aligned} \tag{38}$$

By Lemma 3, the last line is lower-bounded by

$$\begin{aligned}&-\ln\operatorname{tr}\left(\int_{\mathbb{R}} dt\;\beta(t)\left|\left(\prod_j e^{\frac{1+it}{2}\tilde{L}_j}\right)e^{\frac{1+it}{2}\ln(T^*T[\rho])}\right|^2\right) \\ &= -\ln\operatorname{tr}\left(\int_{\mathbb{R}} dt\;\beta(t)\left|\prod_j e^{\frac{1+it}{2}\tilde{L}_j}\right|^2 e^{\ln(T^*T[\rho])}\right) \\ &= -\ln\operatorname{tr}\left(\int_{\mathbb{R}} dt\;\beta(t)\left|\prod_j e^{\frac{1+it}{2}\tilde{L}_j}\right|^2 T^*T[\rho]\right) \\ &= -\ln\operatorname{tr}\left(T^*T\left[\int_{\mathbb{R}} dt\;\beta(t)\left|\prod_j e^{\frac{1+it}{2}\tilde{L}_j}\right|^2\right]\rho\right),\end{aligned} \tag{39}$$

yielding the desired result. □

## V. ASSUMING PROJECTIVE MEASUREMENTS

When considering general scenarios involving uncharacterized measurements, it may not always be valid to assume that they are all projective: for instance, counterexamples have been found for sequential measurements [12] and contextuality scenarios [13]. However, we shall show in this section that for DIQKD as considered in this work, this assumption poses no issues.

We first construct a simultaneous Naimark dilation of all the POVMs, following fairly standard methods (see e.g. [14]). Suppose that Alice and Bob's devices are performing POVMs, i.e. $\Pr(ab|xy) = \operatorname{tr}[(E_{a|x}\otimes E_{b|y})\rho_{AB}]$. To construct the Naimark dilation, we embed an arbitrary state $\rho_{AB}$ in a higher-dimensional Hilbert space via the identification $\rho_{AB} \cong V\rho_{AB}V^*$, where $V$ is the isometry

$$V|\psi\rangle_{AB} = |00\rangle_{\bar{A}\bar{B}}|\psi\rangle_{AB}, \tag{40}$$

with $\bar{A}, \bar{B}$ being Hilbert spaces of dimension equal to the number of measurement outcomes.[6] We then define projectors for Alice via $P_{a|x} = U_x^\dagger(|a\rangle\langle a|\otimes \mathrm{id}_A)U_x$, where $U_x$ are any unitary operators satisfying

$$U_x(|0\rangle_{\bar{A}}|\psi\rangle_A) = \sum_a |a\rangle_{\bar{A}}\sqrt{E_{a|x}}|\psi\rangle_A. \tag{41}$$

Defining $P_{b|y}$ analogously for Bob, it is easily verified that these operators satisfy

$$\operatorname{tr}[(E_{a|x}\otimes E_{b|y})\rho_{AB}] = \operatorname{tr}[(P_{a|x}\otimes P_{b|y})\rho_{AB}], \tag{42}$$

where on the right-hand side we have implicitly embedded $\rho_{AB}$ in the larger Hilbert space. Therefore, one can dilate the POVMs to projective measurements while preserving the constraints.

We shall now argue that for the optimization problem relevant to DI or sDI cryptography (Eq. (1)), this dilation also does not affect the objective function, so it is sufficient to optimize over projective measurements only. This simply follows from the fact that the objective function and constraints in Eq. (1) can be written entirely in terms of the classical-classical-quantum states $(R_{xy}\otimes \mathrm{id}_E)[\rho_{ABE}]$, where $R_{xy}$ are the channels mapping Alice and Bob's quantum states to classical output registers $A_x, B_y$:

$$R_{xy}[\rho_{AB}] = \sum_{ab}|ab\rangle\langle ab|_{A_xB_y}\operatorname{tr}[(E_{a|x}\otimes E_{b|y})\rho_{AB}], \tag{43}$$

for all input pairs $x, y$. By Eq. (42), we see that these are exactly the same channels as would be realised by

[6] We can assume without loss of generality that all measurements have the same number of outcomes, by appending trivial POVM operators to any POVM sets with fewer outcomes.

the projectors $P_{a|x}, P_{b|y}$ (embedding $\rho_{AB}$ in the larger Hilbert space). Therefore, the objective function is indeed invariant under the dilation (the embedding does not affect Eve's system).

(We remark that *a priori*, one might instead wish to consider channels $R'_{xy}$ from $AB$ to $A_xB_yA'B'$, where $A', B'$ are quantum registers storing Alice and Bob's post-measurement states. The constraints and objective function would then be described via the channels $\mathrm{tr}_{A'B'} \circ (R'_{xy} \otimes \mathrm{id}_E)$. However, it is easily verified that $\mathrm{tr}_{A'B'} \circ (R'_{xy} \otimes \mathrm{id}_E) = (\mathrm{tr}_{A'B'} \circ R'_{xy}) \otimes \mathrm{id}_E = R_{xy} \otimes \mathrm{id}_E$, so this produces the same results.)

## VI. DUAL PROBLEM

We shall use the dual of the optimization problem (1) to argue that when applied to DIQKD, our approach yields bounds that are tight up to the use of the generalised Golden–Thompson inequality and NPA hierarchy, except possibly for certain edge cases that would not arise in practical applications.

For brevity, we will again denote the constraints $\left\langle X_{ab|xy}\right\rangle_\psi = \Pr(ab|xy)$ in the form $\left\langle X_j\right\rangle_\psi = \gamma_j$ for $j$ in an index set $\mathcal{J}$, as in Sec. II. Now let $F(\vec{\gamma})$ denote the optimal value of the optimization problem (1), viewed as a function of the constraint values $\vec{\gamma}$. This is not a convex optimization problem, because the constraints are not convex in the standard sense. However, it has the crucial property that $F$ is still a convex function, because we have a "pseudo-convex" behaviour arising from the fact that Eve can always perform classical mixtures of different strategies.[7] This suggests that we can apply some methods from convex analysis. In this section, we will follow conventions in that field and take $F$ to be a function $\mathbb{R}^{|\mathcal{J}|} \to [-\infty, +\infty]$, with the infimum of an empty set being $+\infty$ (this implies $F(\vec{\gamma}) = +\infty$ if and only if $\vec{\gamma}$ is not achievable by any of the states and measurements we consider). It is also conventional to define the "domain" of $F$ to be the set

$$\mathrm{dom}(F) = \{\vec{\gamma} \in \mathbb{R}^{|\mathcal{J}|} \mid F(\vec{\gamma}) < +\infty\}. \tag{44}$$

It is convenient to first rewrite the optimization in the same way as [15]. Specifically, it is noted there that for any pure $\psi_{ABE}$ and projective measurement $A_0$, we have $H(A_0|E) = D(\rho_{AB}||T[\rho_{AB}])$, where $T$ is the channel we used in the context of DIQKD (Eq. (4)). Since for DIQKD we can indeed assume $\psi_{ABE}$ is pure and all measurements are projective, we can conclude

$$F(\vec{\gamma}) = \inf_{(\rho,\vec{X})\in\mathcal{S}_{\vec{\gamma}}} D(\rho||T[\rho]), \tag{45}$$

where $\mathcal{S}_{\vec{\gamma}}$ is the set[8] of all $\rho, \vec{X}$ such that $\langle\vec{X}\rangle_\rho = \vec{\gamma}$. (In the above and subsequent expressions, $\rho$ is to be understood as the state on $AB$ only.)

Let us compare $F$ to the bound given by our approach before the generalized Golden–Thompson inequality is applied, which we can write as (see Eq. (38)):

$$\begin{aligned}\tilde{F}(\vec{\gamma}) &= \sup_{\vec{\lambda}} \inf_{(\rho,\vec{X})\in\mathcal{S}_{\vec{\gamma}}} \left[\langle\vec{\lambda}\cdot\vec{X}\rangle_\rho - \ln\left(\mathrm{tr}\left(e^{\ln(T^*T[\rho])+\vec{\lambda}\cdot\vec{X}}\right)\right)\right] \\ &= \sup_{\vec{\lambda}} \left[\vec{\lambda}\cdot\vec{\gamma} - \sup_{(\rho,\vec{X})\in\mathcal{S}_{\vec{\gamma}}} \ln\left(g\left(\rho, \vec{\lambda}\cdot\vec{X}\right)\right)\right], \end{aligned} \tag{46}$$

where we used the fact that $\langle\vec{X}\rangle_\rho = \vec{\gamma}$ for all states and measurements in $\mathcal{S}_{\vec{\gamma}}$, and introduced the function

$$g(\rho, L) = \mathrm{tr}\left(e^{\ln(T[\rho])+L}\right), \tag{47}$$

using the fact that $T^*T = T$ in the DIQKD setting.

By construction, this is a lower bound: $F \geq \tilde{F}$. We now prove two lemmas that together imply that the reverse inequality $\tilde{F}(\vec{\gamma}) \geq F(\vec{\gamma})$ holds for all $\vec{\gamma}$ in the relative interior of $\mathrm{dom}(F)$, and hence the bound is tight for all such points. This is sufficient to cover practical implementations, since any $\vec{\gamma} \in \mathrm{dom}(F)$ that is not in the relative interior corresponds to a boundary point of the set of distributions allowed by quantum theory, which would not arise in physical implementations with nontrivial noise. (Alternatively, one can restrict Eve's allowed strategies slightly such that the Lemma 5 holds for all $\vec{\gamma} \in \mathbb{R}^{|\mathcal{J}|}$; see the discussion at the end of its proof.)

**Lemma 4.** *For $F$ and $\tilde{F}$ as described in Eq.* (45) *and* (46)*, we have $\tilde{F} \geq G$ where $G$ is the Lagrange dual of the optimization* (45).

---

[7] Specifically: consider any $\vec{\gamma}_0, \vec{\gamma}_1 \in \mathrm{dom}(F)$, and any $\epsilon > 0$. By definition of $F$, there exists a state (and measurements) achieving outcome distribution $\vec{\gamma}_0$ and conditional entropy $H(A_0|E) = h_0$ for some value $h_0 \leq F(\vec{\gamma}_0) + \epsilon$. Doing the same for $\vec{\gamma}_1$, we now note that if Eve has a classical register $E'$ in the state $p|0\rangle\langle 0| + (1-p)|1\rangle\langle 1|$ and uses it to determine which of those strategies to implement (including providing copies of $E'$ to the users' devices so they can implement the corresponding measurements), this yields a strategy that achieves outcome distribution $p\vec{\gamma}_0 + (1-p)\vec{\gamma}_1$ and $H(A_0|EE') = ph_0 + (1-p)h_1$. By definition of $F$, this implies $F(p\vec{\gamma}_0 + (1-p)\vec{\gamma}_1) \leq ph_0 + (1-p)h_1 \leq pF(\vec{\gamma}_0) + (1-p)F(\vec{\gamma}_1) + \epsilon$, proving that $F$ is convex since $\epsilon > 0$ was arbitrary. Notice that this argument uses the fact that there is no bound on the dimension of Eve's side-information.

[8] Strictly speaking, this collection might not be a valid set, depending on the precise specification of the "allowed" states and measurements (for this work, we restrict this to be the union over $n \in \mathbb{N}$ of states and measurements on $\mathbb{C}^n \otimes \mathbb{C}^n$, in which case $\mathcal{S}_{\vec{\gamma}}$ is a valid set, but if we allow arbitrary algebras or Hilbert spaces then some care may be needed). We can address this by noting that Eq. (45) implicitly means $F(\vec{\gamma}) = \inf \mathcal{A}_{\vec{\gamma}}$ where $\mathcal{A}_{\vec{\gamma}}$ is a subset of $\mathbb{R}$ (i.e. a valid set) defined via $\mathcal{A}_{\vec{\gamma}} = \{h \in \mathbb{R} \mid \exists \rho, \vec{X} \text{ s.th. } D(\rho||T[\rho]) = h \text{ and } \mathrm{tr}[\rho\vec{X}] = \vec{\gamma}\}$, with the existence quantifier taken over the class of "allowed" states and measurements. For brevity, however, we continue referring to $\mathcal{S}_{\vec{\gamma}}$ as a set. Alternatively, one could analyze this in terms of the universal representation, as in Sec. VII.

*Proof.* The Lagrange dual is

$$G(\vec{\gamma}) = \sup_{\vec{\lambda}} \inf_{\rho,\vec{X}} D(\rho||T[\rho]) - \vec{\lambda}\cdot\left(\langle\vec{X}\rangle_\rho - \vec{\gamma}\right), \quad (48)$$

where $\inf_{\rho,\vec{X}}$ refers to an infimum over the entire allowed class of states and measurements, not just those in the set $\mathcal{S}_{\vec{\gamma}}$. We first note that for any $\vec{\lambda}$ and finite-dimensional $\vec{X}$, we can follow the derivation in [15] and write

$$\begin{aligned}
&\inf_{\rho} D(\rho||T[\rho]) - \vec{\lambda}\cdot\left(\langle\vec{X}\rangle_\rho - \vec{\gamma}\right) && (49)\\
&= \inf_{\rho,\sigma} D(\rho||T[\sigma]) - \vec{\lambda}\cdot\left(\langle\vec{X}\rangle_\rho - \vec{\gamma}\right) && (50)\\
&= \inf_{\sigma} -\operatorname{tr}\left(e^{\ln(T[\sigma])+\vec{\lambda}\cdot\vec{X}-\mathbb{I}}\right) + \vec{\lambda}\cdot\vec{\gamma} && (51)\\
&= \vec{\lambda}\cdot\vec{\gamma} - \sup_{\rho}\frac{1}{e}g\left(\rho,\vec{\lambda}\cdot\vec{X}\right), && (52)
\end{aligned}$$

where in the last line we have relabelled $\sigma$ as $\rho$ (since it is merely a "dummy variable" in the optimization). Hence we can rewrite the expression for $G$:

$$\begin{aligned}
G(\vec{\gamma}) &= \sup_{\vec{\lambda}}\inf_{\vec{X}}\inf_{\rho} D(\rho||T[\rho]) - \vec{\lambda}\cdot\left(\langle\vec{X}\rangle_\rho - \vec{\gamma}\right) && (53)\\
&= \sup_{\vec{\lambda}}\left[\vec{\lambda}\cdot\vec{\gamma} - \sup_{\rho,\vec{X}}\frac{1}{e}g\left(\rho,\vec{\lambda}\cdot\vec{X}\right)\right]. && (54)
\end{aligned}$$

Now note that by the inequality $\ln x \leq x/e$, we have

$$\sup_{(\rho,\vec{X})\in\mathcal{S}_{\vec{\gamma}}} \ln\left(g\left(\rho,\vec{\lambda}\cdot\vec{X}\right)\right) \leq \sup_{\rho,\vec{X}}\frac{1}{e}g\left(\rho,\vec{\lambda}\cdot\vec{X}\right), \quad (55)$$

since the supremum on the left is over a smaller set. Referring back to Eq. (46), we hence see that $\tilde{F} \geq G$. □

**Lemma 5.** *For $F$ as described in Eq.* (45)*, we have $G(\vec{\gamma}) = F(\vec{\gamma})$ for all $\vec{\gamma}$ in the relative interior of* dom$(F)$*, where $G$ is the Lagrange dual of the optimization* (45)*.*

*Proof.* We will argue via the (Legendre-Fenchel) conjugate of $F$, denoted as $F^*$. Abstractly, the $F$ we consider here is a constrained optimization of the form

$$\begin{aligned}
F(\vec{\gamma}) = &\inf_{x\in D} f(x)\\
&\text{s.th. } \Gamma_j(x) = \gamma_j \quad \forall j\in\mathcal{J},
\end{aligned} \quad (56)$$

where $D$ is some optimization domain (which could in principle be a class rather than a set, though we will continue using set notation for it), and $f$ and $\Gamma_j$ are functions (or class functions) $D\to\mathbb{R}$. In such cases, the Lagrange dual of the optimization is equal to the biconjugate $F^{**}$. For completeness, we provide a proof here (that applies even for nonconvex optimizations), based on [16] Sec. 5.1.6.

First, recall that since $f(x)\in\mathbb{R}$, dom$(F)$ is in fact equal to the set

$$\{\vec{\gamma}\in\mathbb{R}^{|\mathcal{J}|} \mid \exists x\in D \text{ s.th. } \vec{\Gamma}(x) = \vec{\gamma}\}. \quad (57)$$

This implies (in the following, all suprema/infima without explicit domains are over $\mathbb{R}^{|\mathcal{J}|}$):

$$\begin{aligned}
-F^*(\vec{\lambda}) &= \inf_{\vec{\gamma}}\left[F(\vec{\gamma}) - \vec{\lambda}\cdot\vec{\gamma}\right] && (58)\\
&= \inf_{\vec{\gamma}\in\mathrm{dom}(F)}\left[F(\vec{\gamma}) - \vec{\lambda}\cdot\vec{\gamma}\right] && (59)\\
&= \inf_{x\in D}\left[F(\vec{\Gamma}(x)) - \vec{\lambda}\cdot\vec{\Gamma}(x)\right] && (60)\\
&= \inf_{x\in D}\left[f(x) - \vec{\lambda}\cdot\vec{\Gamma}(x)\right]. && (61)
\end{aligned}$$

(The last step follows from the definition of $F$, which implies that for any $\epsilon > 0$ and $x\in D$, there exists $x'\in D$ such that $\vec{\Gamma}(x) = \vec{\Gamma}(x')$ and $F(\vec{\Gamma}(x)) + \epsilon \geq f(x')$. It is slightly tedious but straightforward to verify that this implies (60) $\geq$ (61). The reverse inequality clearly holds, and hence both are equal.) Hence for any $\vec{\gamma}\in\mathbb{R}^{|\mathcal{J}|}$, we indeed have

$$\begin{aligned}
F^{**}(\vec{\gamma}) &= \sup_{\vec{\lambda}}\left[\vec{\lambda}\cdot\vec{\gamma} - F(\vec{\lambda})\right] && (62)\\
&= \sup_{\vec{\lambda}}\left[\vec{\lambda}\cdot\vec{\gamma} + \inf_{x\in D}\left[f(x) - \vec{\lambda}\cdot\vec{\Gamma}(x)\right]\right] && (63)\\
&= \sup_{\vec{\lambda}}\inf_{x\in D}\left[f(x) - \vec{\lambda}\cdot\vec{\Gamma}(x) + \vec{\lambda}\cdot\vec{\gamma}\right] && (64)\\
&= G(\vec{\gamma}), && (65)
\end{aligned}$$

where $G$ is the Lagrange dual of the optimization in $F$.

The biconjugate $F^{**}$ is always a (convex and lower semicontinuous) lower bound on $F$. For convex $F$ in particular, we have $F^{**}(\vec{\gamma}) = F(\vec{\gamma})$ for all $\vec{\gamma}$ in the relative interior of dom$(F)$ (see e.g. [17] Prop. 3.2.6 together with Prop. 2.2.2). Since the $F$ we consider in DIQKD is convex, as previously discussed, we indeed have $G(\vec{\gamma}) = F(\vec{\gamma})$ for such points as claimed.

We could gain some geometric insight into the behaviour of points on the boundary by considering the set $\mathcal{A}\subseteq\mathbb{R}^{|\mathcal{J}|+1}$ defined as (see [16])

$$\mathcal{A} = \{(\vec{\gamma},t) \mid \exists x\in D \text{ s.th. } \Gamma_j(x) = \gamma_j, f(x)\leq t\}. \quad (66)$$

Essentially, $\mathcal{A}$ is the union of the strict epigraph of $F$ with some subset of the graph of $F$. In our specific (DIQKD) context, $\mathcal{A}$ is convex by a strategy-mixing argument as previously described. If $\mathcal{A}$ were closed as well, then we would have $F^{**} = F$ (see [16] Sec. 3.3.2). However, the question of whether $\mathcal{A}$ is closed seems to depend on whether the set of quantum correlations is closed in a given Bell scenario, which is rather subtle and outside the scope of this work. (There may be ways to modify the set of Eve's allowed strategies such that $\mathcal{A}$ is both convex and closed, for instance if we restrict Eve to mixtures of $d$-dimensional strategies for a large but fixed value $d$, with a classical ancilla $E'$ to record which strategy was used.) □

We remark that in this work we have described how to bound $\tilde{F}$, but the same methods could have been applied

to bound the Lagrange dual $G$ in the form (54), since they are essentially describing ways to bound the function $g$. However, by recalling the inequality $\ln x \leq x/e$, we can see from the expressions (46) and (54) that when the same methods are applied in both cases to bound $g$, the bound resulting from $\tilde{F}$ is always at least as good as the one resulting from $G$,[9] which is perhaps slightly surprising since we have a tightness argument for $G$ (Lemma 5), whereas the inequalities involved in deriving $\tilde{F}$ do not appear tight *a priori*.

Lastly, we remark that our final bound (Eq. (17) with $\langle K\rangle_\rho$ bounded in terms of $\vec{\gamma}$ using the SDP method as described) is convex with respect to $\vec{\gamma}$. This follows from the fact that the optimal value of a maximization SDP is a concave function of the constraint values $\vec{\gamma}$, and $-\ln$ is a convex nonincreasing function, which implies their composition is a convex function of $\vec{\gamma}$. Hence our final bound is also a convex function of $\vec{\gamma}$ (the $\langle L\rangle_\rho$ term is linear in $\vec{\gamma}$ and hence trivially convex). This property is important in some applications, such as the entropy accumulation theorem [2–4]. If one needs to impose the stronger requirement that the bound is affine, then note that if we pick any particular $\vec{\lambda}$ in Eq. (46) rather than taking the supremum, and relax the inner optimization to $\sup_{\rho,\vec{X}}$, we get an affine lower bound with gradient $\vec{\lambda}$. In addition, this $\vec{\lambda}$ essentially describes a single Bell expression that certifies the same amount of entropy as can be certified by all the original constraints using this choice of $\vec{\lambda}$ (in the relaxed optimization). However, this approach (relaxing the inner optimization) comes with the drawback that it can potentially make the final bound worse.

## VII. NON-COMMUTATIVE POLYNOMIAL OPTIMIZATION ON $C^*$-ALGEBRAS AND SDP HIERARCHIES

When studying device-independent scenarios, there can potentially be some variability in specifying the exact class of states and measurements to consider — for instance, whether one restricts the analysis to finite-dimensional Hilbert spaces with a tensor-product structure (as in this work), or whether one allows arbitrary Hilbert spaces and merely requires some measurements to commute. In the following, we outline a framework that encapsulates a rather general range of possibilities, within which we can restrict ourselves to narrower classes as necessary. (See footnote 8 for a slightly different perspective.)

To begin with, we shall assume there exists enough structure in our problem description to have a (unital) C*-algebra $\mathcal{A}$ that abstractly describes all observables $X_j$ we have to take into account. Whenever a particular such algebra $\mathcal{A}$ is provided, the set of all states $\mathcal{S}(\mathcal{A})$ is a well defined object given by the set of all positive normalized linear functionals [18]. Using the Gelfand-Naimark-Segal construction we can then assign representations $\pi_\rho : \mathcal{A} \to \mathcal{B}(\mathcal{H})$ to states which then allow us to speak about the $X_j$ as an explicit set of bounded operators on a specified Hilbert space, for which a functional calculus exists such that the computations done in the last section would hold.

Building on this, one can additionally consider the universal representation $\mathcal{U}$ of $\mathcal{A}$, which is simply the direct sum over all representations $\pi_\rho$, i.e.

$$\mathcal{U}(\mathcal{A}) = \bigoplus_{\rho\in\mathcal{S}(\mathcal{A})} \pi_\rho(\mathcal{A}). \tag{67}$$

We will hence interpret device-independent formulations of the optimization problem (1) to be an optimization over this underlying object, where we extended the functional calculus from the $\pi_\rho$ to $\mathcal{U}$. Furthermore we have the identification

$$\rho\left(\mathcal{U}(X_j)\right) = \rho(\pi_\rho(X_j)) = \langle X_j\rangle_\rho = \operatorname{tr}\left(\rho X_j\right). \tag{68}$$

To restrict to narrower classes of possibilities, one would simply need to specify that only certain blocks in the direct sum should be considered (for instance, only finite-dimensional representations).

We now turn to a description of non-commutative polynomial optimizations in general. Whenever we fix a list $X = \{X_1, \dots, X_n\}$, in the following context also referred to as an alphabet $X$ of letters $X_j$, we can define the set of all possible concatenations of letters, i.e.

$$\mathcal{W} = \{\mathbb{I}, X_1, X_2, \dots, X_1X_2 \dots X_1X_2X_3 \dots\}. \tag{69}$$

We refer to this as the set of words, and index it with some index-set $\mathcal{I}$. A non-commutative polynomial $P(X)$ with coefficients $c_{ij} \in \mathbb{C}$ is then given as a finite linear combination of words $w_i, w_j \in \mathcal{W}$, i.e.

$$P(X) = \sum_{ij\in\Omega} c_{ij} w_i w_j^*, \tag{70}$$

for some set $\Omega \subseteq \mathcal{I}$. (We use two indices $i, j$ to index the terms of the polynomial because it will subsequently be convenient to consider a matrix of coefficients $c_{ij}$.) We will call $P$ hermitian if $c_{ij} = \overline{c}_{ji}$ holds for all $ij$.

We are now in a position to interpret an expression such as the expansion of $K$ in (26) as a non-commutative polynomial $P(X)$ arising from some computation done in the representation $\mathcal{U}$ which is then evaluate on a particular state $\rho$ via (68). Additionally we can also collect the

---

[9] Noting that we have $g(\rho, \vec{\lambda}\cdot\vec{X} + \alpha\mathbb{I}) = e^\alpha\, g(\rho, \vec{\lambda}\cdot\vec{X})$ for any $\alpha \in \mathbb{R}$, and exploiting the "normalization condition" described in Sec. VIII, one can show that the bounds provided by $\tilde{F}$ and $G$ are in fact the same up to the difference between $\sup_{(\rho,\vec{X})\in\mathcal{S}_{\vec{\gamma}}}$ and $\sup_{\rho,\vec{X}}$. Essentially, the optimisation over $\vec{\lambda}$ implicitly parametrizes a family of affine upper bounds on $\ln\big(g(\rho, \vec{\lambda}\cdot\vec{X})\big)$, and the envelope of these affine bounds returns precisely the ln function.

constraints $\langle X_j \rangle_\rho = \gamma_j$ and some other algebraic constraints, which are not trivially covered as identity in $\mathcal{A}$, by a list of further constraints $\langle Q_k(X) \rangle_\rho \geq \alpha_k$ that are expressed as non-commutative polynomials $Q_k$. (In a generic non-commutative polynomial optimization, it may not be clear *a priori* whether an imposed constraint, for example $X_1 + X_2 = \mathbb{I}$, should be fulfilled on the level of an operator identity or only for a particular state, i.e. as $\langle X_1 \rangle_\rho + \langle X_2 \rangle_\rho = 1$, which is weaker. However, in the context of quantum theory this is determined by the chosen postulates.)

At the end we arrive at a point where we can formulate the task of finding a device-independent bound on the expectation $\langle K \rangle_\rho$ from (17) as an optimization problem

$$\begin{aligned} \inf \quad & \langle P(X) \rangle_\rho \\ \text{s.th.:} \quad & \langle Q_k(X) \rangle_\rho \geq \alpha_k \qquad \forall k \\ & \rho \in \mathcal{S}(\mathcal{A}) \end{aligned} \tag{71}$$

on objects defined in the aforementioned sense.

By introducing the matrix $\Gamma_\Omega^\rho$ with entries

$$(\Gamma_\Omega^\rho)_{ij} = \langle w_i w_j^* \rangle_\rho, \tag{72}$$

which is also called the moment matrix of $X$ or the representing GNS matrix of $\rho$ on $\mathcal{W}|_\Omega$, we can rewrite

$$\langle P(X) \rangle_\rho = \sum_{ij \in \Omega} c_{ij} \langle w_i w_j^* \rangle_\rho = \operatorname{tr}\left(C_\Omega^P \Gamma_\Omega^\rho\right). \tag{73}$$

Let $\mathcal{C}_\Omega$ be the set of indices $k$ such that the polynomial $Q_k(X)$ only involves terms from the set $\Omega$. For any $k \in \mathcal{C}_\Omega$, we can analogously write

$$\langle Q_k(X) \rangle_\rho = \operatorname{tr}\left(C_\Omega^{Q_k} \Gamma_\Omega^\rho\right), \tag{74}$$

for some matrix $C_\Omega^{Q_k}$. Then a lower bound on (71) (differing only in that some constraints are omitted) is

$$\begin{aligned} \inf \quad & \operatorname{tr}\left(C_\Omega^P \Gamma_\Omega^\rho\right) \\ \text{s.th.:} \quad & \operatorname{tr}\left(C_\Omega^{Q_k} \Gamma_\Omega^\rho\right) \geq \alpha_k \qquad \forall k \in \mathcal{C}_\Omega \\ & \rho \in \mathcal{S}(\mathcal{A}), \end{aligned} \tag{75}$$

which is an optimization of linear matrix functionals over the set

$$\Xi_\Omega = \{\Gamma_\Omega^\rho | \rho \in \mathcal{S}(\mathcal{A})\} \tag{76}$$

of all valid matrices $\Gamma_\Omega^\rho$.

It is well known that a matrix like $\Gamma_\Omega^\rho$ is a positive matrix whenever $\rho$ is a positive functional. We therefore have that $\Xi_\Omega$ is a subset of $\mathcal{P}_n^+$ the positive $n \times n$ matrices with $n = |\Omega|$. This observation [6] directly suggests to relax the optimization problem (75) by extending the optimization from $\Xi_\Omega$ to $\mathcal{P}_n^+$, which will then result in the semidefinite program

$$\begin{aligned} \inf \quad & \operatorname{tr}\left(C_\Omega^P \Gamma\right) \\ \text{s.th.:} \quad & \operatorname{tr}\left(C_\Omega^{Q_k} \Gamma\right) \geq \alpha_k \qquad \forall k \in \mathcal{C}_\Omega \\ & \Gamma \in \mathcal{P}_n^+. \end{aligned} \tag{77}$$

Note that in constructing this relaxed optimization, we have only required that the domain $\Omega$ is large enough to represent $P$, but not necessarily all algebraic constraints $Q_k$ in the original optimization (71). By expanding the set $\Omega$, we could include more and more constraints $Q_k$ expressing the structure of $\mathcal{A}$. For our original formulation (71), this does not make any difference since all such constraints are included. For the relaxation (77), however, this will have an impact. We therefore get a hierarchy of semidefinite programs by subsequently replacing $\Omega$ in (77) with a sequence of sets $\Omega \subset \Omega' \subset \Omega'' \dots \subset I$ whilst incorporating more and more structural constraints from $\mathcal{A}$ by adding new $Q_k$.

In an explicit application of this technique, the optimal choice of those new constraints and a suitable sequence of sets is highly case-dependent and influenced by the computational resources that could be spent.

## VIII. DETAILS FOR NUMERICAL WORK

By level $n$ of the NPA hierarchy we always mean the "global level", i.e. the rows/columns of the NPA matrix are indexed by all the operators consisting of products of $n$ or fewer projectors. This is in contrast to "local level" $n$, where the index operators are all the operators consisting of products of $n$ or fewer projectors per party. Essentially, local level $n$ is equal to global level $2n$ with some index operators removed (namely, all those which have more than $n$ projectors by a single party). The local level concept can be slightly extended by having different local levels for Alice and Bob.

In our approach, high levels of the NPA hierarchy are required in order to have all the terms in Eq. (26) appearing in the NPA matrix (unless we simplify by restricting some of the coefficients $\lambda_{ab|xy}$ to be zero). To cope with this, we used the simplification that one projector per measurement can be omitted, by using the relation $\sum_c P_{c|z} = \mathbb{I}$ to write one of the projectors $P_{c|z}$ in terms of the others.

For scenarios with 2 inputs per party, global level 6 is sufficient to capture all the terms in Eq. (26) (for some choices of the operator product order, at least), with the NPA matrix having size $85 \times 85$ when the above simplification is implemented. In principle, local level 5 for Alice with local level 3 for Bob is also sufficient (while producing a slightly smaller NPA matrix of size $77 \times 77$), since the terms in Eq. (26) have basically equal numbers of projectors from each party, apart from the asymmetry introduced by the channel $T$. However, the resulting bounds we obtained were slightly but noticeably worse than those for global level 6, to the extent that it is no longer able to outperform the bound in [9], at least as far as we were able to optimize the coefficients $\lambda_{ab|xy}$.

We also note that some algebraic constraints on the projectors can be used to reduce the number of coefficients $\lambda_{ab|xy}$ to optimize over. For instance, we can use the normalization conditions $\sum_{ab} P_{a|x} \otimes P_{b|y} = \mathbb{I}$ to

eliminate one coefficient per input pair $(x, y)$, as follows. Consider any set of values for $\lambda_{ab|xy}$. Pick some specific input pair $(\tilde{x}, \tilde{y})$ and a real number $\alpha \in \mathbb{R}$, and define a new set of coefficients as follows:

$$\lambda'_{ab|xy} = \begin{cases} \lambda_{ab|xy} - \alpha & \text{for } (x, y) = (\tilde{x}, \tilde{y}), \\ \lambda_{ab|xy} & \text{otherwise.} \end{cases} \tag{78}$$

We now show that the coefficients $\lambda'_{ab|xy}$ yield the same bound as the coefficients $\lambda_{ab|xy}$. Denote the operators constructed from the coefficients $\lambda'_{ab|xy}$ (in the sense of Corollary 1) as $L'$ and $K'$. First, it is easy to see that $\langle L' \rangle_\rho = \langle L \rangle_\rho - \alpha$ due to the normalization conditions. Similarly, we also have

$$\begin{aligned} &\left| \prod_{xy} \left( \sum_{ab} e^{\frac{1+it}{2} \lambda'_{ab|xy}} P_{a|x} \otimes P_{b|y} \right) \right|^2 \\ =&\left| e^{-\frac{1+it}{2}\alpha} \prod_{xy} \left( \sum_{ab} e^{\frac{1+it}{2} \lambda_{ab|xy}} P_{a|x} \otimes P_{b|y} \right) \right|^2 \\ =&e^{-\alpha} \left| \prod_{xy} \left( \sum_{ab} e^{\frac{1+it}{2} \lambda_{ab|xy}} P_{a|x} \otimes P_{b|y} \right) \right|^2, \end{aligned} \tag{79}$$

which implies that $\langle K' \rangle_\rho = e^{-\alpha} \langle K \rangle_\rho$ and thus $\langle L' \rangle_\rho - \ln \langle K' \rangle_\rho = \langle L \rangle_\rho - \ln \langle K \rangle_\rho$, as claimed. Notice that if we choose $\alpha$ to be equal to one of the $\lambda_{ab|\tilde{x}\tilde{y}}$ values, this procedure yields a new set of coefficients $\lambda'_{ab|xy}$ that gives the same bound, but with the corresponding $\lambda'_{ab|\tilde{x}\tilde{y}}$ value equal to zero. In summary, this implies that for each input pair $(x, y)$, we can set one coefficient $\lambda_{ab|xy}$ to be zero without loss of generality.

It might appear that something similar could be done with the no-signalling conditions; namely, if we pick some specific $\tilde{a}, \tilde{x}, \tilde{y}, \tilde{y}'$, they must satisfy $\sum_b P_{\tilde{a}|\tilde{x}} \otimes P_{b|\tilde{y}} = \sum_b P_{\tilde{a}|\tilde{x}} \otimes P_{b|\tilde{y}'}$, since $\sum_b P_{b|y} = \mathbb{I}$ for any $y$. (Analogous conditions hold for summations over Alice's outputs $a$. The statements we derive below also cover those no-signalling conditions, as well as the no-signalling conditions in "marginal form", $\sum_b P_{\tilde{a}|\tilde{x}} \otimes P_{b|\tilde{y}} = P_{\tilde{a}|\tilde{x}} \otimes \mathbb{I}$.) However, this approach runs into a subtle difficulty. To see this, consider how one could try to proceed in a manner similar to the use of the normalization conditions: take any set of values for $\lambda_{ab|xy}$, pick some $\alpha \in \mathbb{R}$, and define

$$\lambda'_{ab|xy} = \begin{cases} \lambda_{ab|xy} - \alpha & \text{for } (a, x, y) = (\tilde{a}, \tilde{x}, \tilde{y}), \\ \lambda_{ab|xy} + \alpha & \text{for } (a, x, y) = (\tilde{a}, \tilde{x}, \tilde{y}'), \\ \lambda_{ab|xy} & \text{otherwise.} \end{cases} \tag{80}$$

Then by the no-signalling conditions, we have $\langle L' \rangle_\rho = \langle L \rangle_\rho$. As for the operator product $\prod_{xy}$ in $K'$, the term with index $(\tilde{x}, \tilde{y})$ has the form[10]

$$\begin{aligned} &\exp\left( \sum_{ab} \frac{1+it}{2} \lambda'_{ab|\tilde{x}\tilde{y}} P_{a|\tilde{x}} \otimes P_{b|\tilde{y}} \right) \\ =&\exp\left( \sum_{ab} \frac{1+it}{2} \lambda_{ab|\tilde{x}\tilde{y}} P_{a|\tilde{x}} \otimes P_{b|\tilde{y}} \right) \times \\ &\exp\left( -\sum_{b} \frac{1+it}{2} \alpha P_{\tilde{a}|\tilde{x}} \otimes P_{b|\tilde{y}} \right), \end{aligned} \tag{81}$$

where the product of the two exponentials in the last line could also be taken in the reverse order (because the operators $P_{a|\tilde{x}} \otimes P_{b|\tilde{y}}$ for different $a, b$ all commute). Similarly, the term with index $(\tilde{x}, \tilde{y}')$ has the form

$$\begin{aligned} &\exp\left( \sum_{ab} \frac{1+it}{2} \lambda'_{ab|\tilde{x}\tilde{y}'} P_{a|\tilde{x}} \otimes P_{b|\tilde{y}'} \right) \\ =&\exp\left( \sum_{ab} \frac{1+it}{2} \lambda_{ab|\tilde{x}\tilde{y}'} P_{a|\tilde{x}} \otimes P_{b|\tilde{y}'} \right) \times \\ &\exp\left( \sum_{b} \frac{1+it}{2} \alpha P_{\tilde{a}|\tilde{x}} \otimes P_{b|\tilde{y}'} \right), \end{aligned} \tag{82}$$

where the product of the two exponentials in the last line could also be taken in the reverse order. All the other terms in the product remain the same as they were with the coefficients $\lambda_{ab|xy}$. We now observe that if the operator product is ordered such that the terms $(\tilde{x}, \tilde{y})$ and $(\tilde{x}, \tilde{y}')$ are next to each other, we would have $K' = K$ because the no-signalling conditions imply that the terms involving $\alpha$ cancel each other out. Hence in such a case, the entropy bound would be invariant under the substitution $\lambda_{ab|xy} \to \lambda'_{ab|xy}$. However, if the operator product is *not* ordered such that those terms are next to each other, then the $\alpha$-dependent terms do not cancel, and it seems possible to have $\langle K' \rangle_\rho \neq \langle K \rangle_\rho$ as a result. In summary, whether a substitution based on the no-signalling conditions leaves the bound invariant depends on the ordering of the operator product when constructing $K$.

When implementing our approach in a context where the constraints are linear combinations of the probabilities instead of simply the form in (1), the above discussion implies that although we can rewrite or eliminate constraints using the normalization conditions while leaving our final bounds invariant, this may not necessarily be true when using the no-signalling conditions. In particular, this means it is possible that the bounds given by our approach might *not* be invariant if we replace the constraints in terms of probabilities with constraints in terms of the Collins-Gisin parametrization [19] (which makes

[10] Here it is more illustrative to consider the terms before Eq. (23) is applied.

use of both the normalization and no-signalling conditions to reduce the number of terms). As tentative support for this possibility, we were unable to reproduce the results in the main text when only imposing constraints in terms of the Collins-Gisin parametrization (though it is possible that this might have simply resulted from the numerical search not finding the optimal bound).

[1] W. F. Stinespring, P. Am. Math. Soc. **6**, 211 (1955).
[2] R. Arnon-Friedman, F. Dupuis, O. Fawzi, R. Renner, and T. Vidick, Nat. Commun. **9**, 459 (2018).
[3] F. Dupuis, O. Fawzi, and R. Renner, arXiv preprint arXiv:1607.01796 (2016).
[4] P. J. Brown, S. Ragy, and R. Colbeck, arXiv preprint arXiv:1810.13346 (2018).
[5] D. Sutter, M. Berta, and M. Tomamichel, Commun. Math. Phys. **352**, 37 (2017).
[6] M. Navascués, S. Pironio, and A. Acín, New J. Phys. **10**, 073013 (2008).
[7] A. Acín, S. Massar, and S. Pironio, Phys. Rev. Lett. **108**, 100402 (2012).
[8] J. Briët and P. Harremoës, Phys. Rev. A **79**, 052311 (2009).
[9] S. Pironio, A. Acin, N. Brunner, N. Gisin, S. Massar, and V. Scarani, New J. Phys. **11**, 045021 (2009).
[10] V. Scarani and R. Renner, in *Theory of Quantum Computation, Communication, and Cryptography*, edited by Y. Kawano and M. Mosca (Springer Berlin Heidelberg, Berlin, Heidelberg, 2008) pp. 83–95.
[11] T. Vértesi, S. Pironio, and N. Brunner, Phys. Rev. Lett. **104**, 060401 (2010).
[12] C. Budroni, T. Moroder, M. Kleinmann, and O. Gühne, Phys. Rev. Lett. **111**, 020403 (2013).
[13] C. Heunen, T. Fritz, and M. L. Reyes, Phys. Rev. A **89**, 032121 (2014).
[14] M. A. Nielsen and I. L. Chuang, *Quantum Computation and Quantum Information* (Cambridge University Press, New York, 2010).
[15] P. J. Coles, E. M. Metodiev, and N. Lütkenhaus, Nat. Commun. **7**, 11712 (2016).
[16] S. Boyd and L. Vandenberghe, *Convex Optimization* (Cambridge University Press, 2004).
[17] A. Sabourin and P. Bianchi, "Convex analysis (lecture notes)," (2014).
[18] S. Sakai, *C*-algebras and W*-algebras* (Springer, Berlin, Heidelberg, 1971).
[19] D. Collins and N. Gisin, Journal of Physics A: Mathematical and General **37**, 1775 (2004).
